# Supplementary material for: ixi-sLM: On-Device sLM for AI Call Agent Service
Source: arXiv:2610.19382 source file (2026-10-14)
Supplement: Supplementary file 1 [file appendix_power.tex]

\begin{table}[H]
\centering
\caption{
Per-call Energy (mAh) by phase, CPU vs.\ NPU.
}
\label{tab:app:ondevice_perf_power}
\vspace{1em}
\begin{tabular}{l ccc}
\toprule
\textbf{Stage} & \textbf{Prefill} & \textbf{Decode} & \textbf{Total} \\
\midrule
CPU & 4.42 & 3.37 & 7.79 \\
NPU & 0.26 & 1.53 & 1.79 \\
\bottomrule
\end{tabular}

\end{table}
